# Supplementary material for: FastComposer: Tuning-Free Multi-Subject Image Generation with Localized Attention
Source: arXiv:2305.10431 source file (2023-05-21)
Supplement: Supplementary file 1 [file supplement.tex]

\documentclass{article}

% if you need to pass options to natbib, use, e.g.:
%     \PassOptionsToPackage{numbers, compress}{natbib}
% before loading neurips_2023

% ready for submission
\usepackage{neurips_2023}

% to compile a preprint version, e.g., for submission to arXiv, add add the
% [preprint] option:
%     \usepackage[preprint]{neurips_2023}

% to compile a camera-ready version, add the [final] option, e.g.:
%     \usepackage[final]{neurips_2023}

% to avoid loading the natbib package, add option nonatbib:
%    \usepackage[nonatbib]{neurips_2023}

\usepackage[utf8]{inputenc} % allow utf-8 input
\usepackage[T1]{fontenc}    % use 8-bit T1 fonts
\usepackage{hyperref}       % hyperlinks
\usepackage{url}            % simple URL typesetting
\usepackage{booktabs}       % professional-quality tables
\usepackage{amsfonts}       % blackboard math symbols
\usepackage{nicefrac}       % compact symbols for 1/2, etc.
\usepackage{microtype}      % microtypography
\usepackage{xcolor}         % colors

\title{FastComposer: Tuning-Free Multi-Subject Image Generation with Localized Attention}

% The \author macro works with any number of authors. There are two commands
% used to separate the names and addresses of multiple authors: \And and \AND.
%
% Using \And between authors leaves it to LaTeX to determine where to break the
% lines. Using \AND forces a line break at that point. So, if LaTeX puts 3 of 4
% authors names on the first line, and the last on the second line, try using
% \AND instead of \And before the third author name.

\author{%
  David S.~Hippocampus\thanks{Use footnote for providing further information
    about author (webpage, alternative address)---\emph{not} for acknowledging
    funding agencies.} \\
  Department of Computer Science\\
  Cranberry-Lemon University\\
  Pittsburgh, PA 15213 \\
  \texttt{hippo@cs.cranberry-lemon.edu} \\
  % examples of more authors
  % \And
  % Coauthor \\
  % Affiliation \\
  % Address \\
  % \texttt{email} \\
  % \AND
  % Coauthor \\
  % Affiliation \\
  % Address \\
  % \texttt{email} \\
  % \And
  % Coauthor \\
  % Affiliation \\
  % Address \\
  % \texttt{email} \\
  % \And
  % Coauthor \\
  % Affiliation \\
  % Address \\
  % \texttt{email} \\
}

\begin{document}

\maketitle

\section{Broader Impact.} %move to appendix 
FastComposer provides a fast and effective approach to personalized multi-subject text-to-image generation, thus democratizing AI-driven content creation by reducing the demand for computational resources and hardware. 
However, the utilization of this model may lead to unexpected consequences.
For instance, the simplified process of creating personalized multi-subject images could enable malicious activities such as the production of deepfakes or other deceptive content. 
Concerns may also arise regarding data privacy and consent in the context of using reference subjects to generate new images.
It is critical that the deployment of such methods is approached with a keen awareness of ethical considerations and their potential societal impacts.
In response to these challenges, the advancement of deepfake detection methods~\cite{dolhansky2020deepfake} could provide a countermeasure, ensuring that image generation techniques are used responsibly and beneficially for society.

\section{Baseline Details}

\section{Evaluation Text Prompts}

\small
\bibliographystyle{plain}
\bibliography{reference}

\end{document}
