# Supplementary material for: FastComposer: Tuning-Free Multi-Subject Image Generation with Localized Attention
Source: arXiv:2305.10431 source file (2023-05-21)
Supplement: Supplementary file 2 [file 8_appendix.tex]

\begin{figure*}[t]
    \centering
    \includegraphics[width=\linewidth]{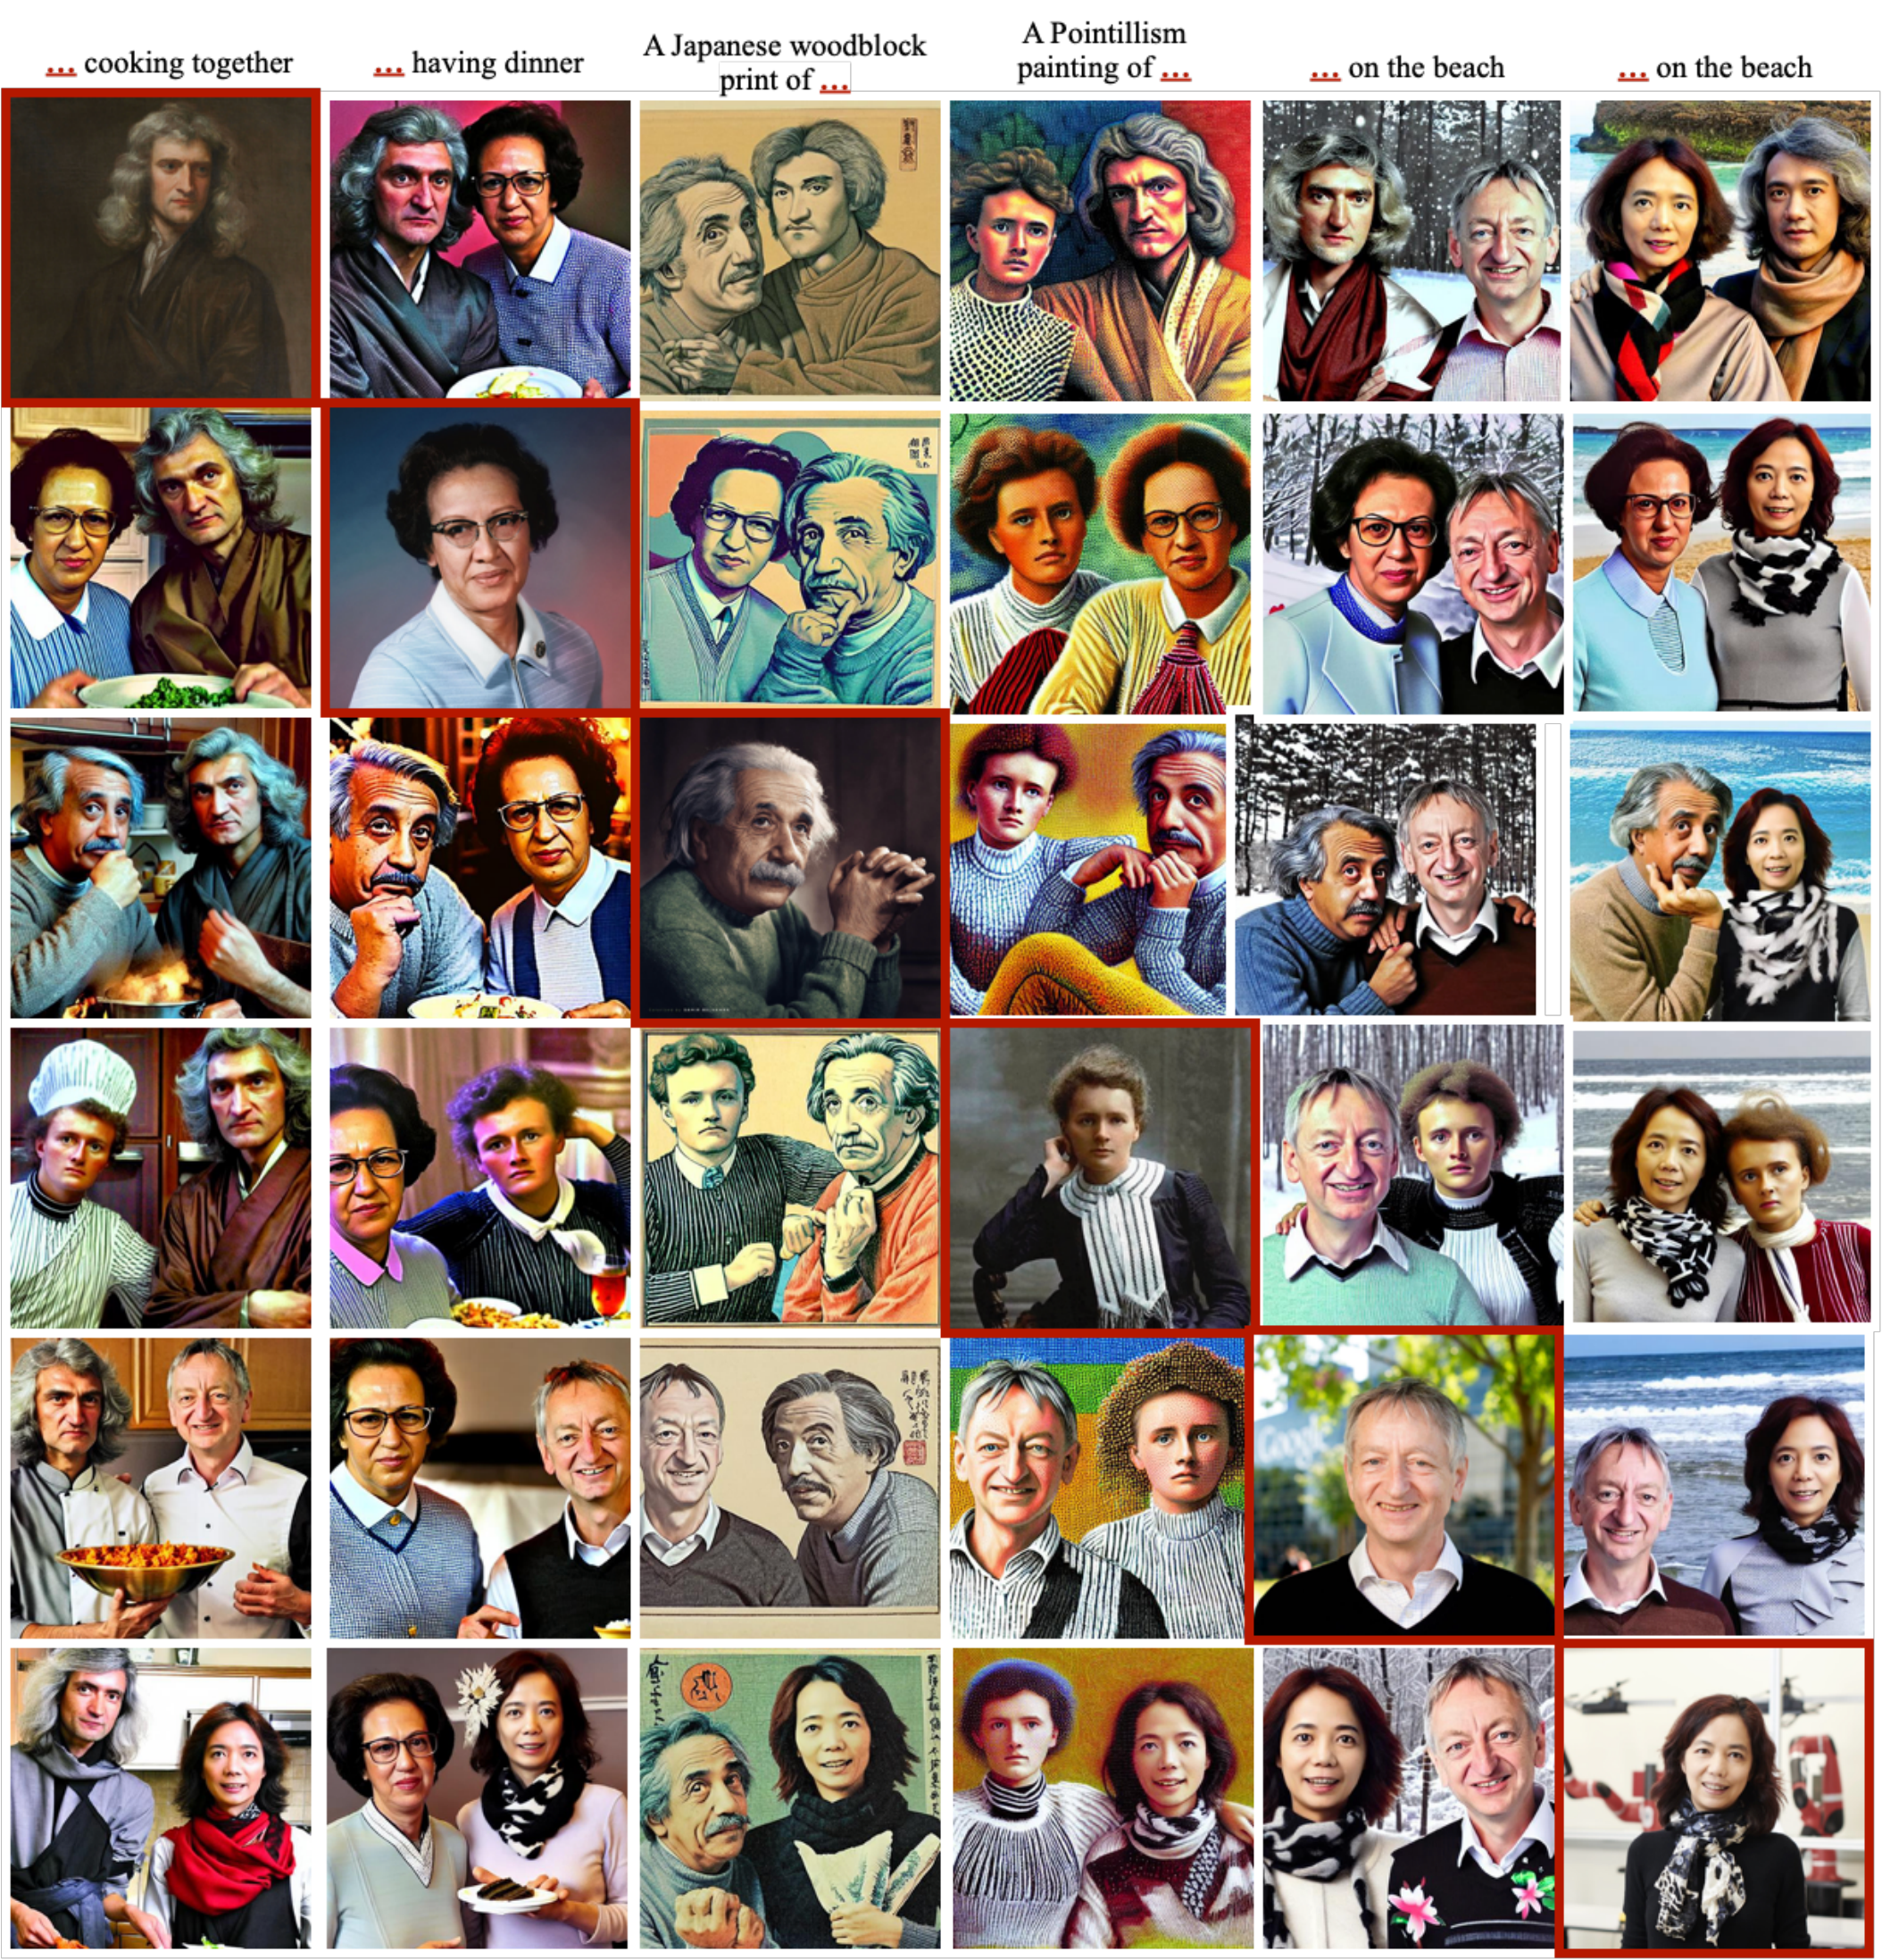}
    \caption{}
    \label{fig:1}
\end{figure*}
